# Supplementary material for: Is Your LiDAR Placement Optimized for 3D Scene Understanding?
Source: arXiv:2403.17009 source file (2024-10-30)
Supplement: Supplementary file 1 [file toc.tex]

\section*{Appendix}
\begin{itemize}

    \item \textcolor{eccvblue}{\textbf{6. \nameref{sec:place3d}}} \dotfill \pageref{sec:place3d}
    \begin{itemize}
        \item \textcolor{eccvblue}{6.1 \nameref{subsec:stats}} \dotfill \pageref{subsec:stats}
        \item \textcolor{eccvblue}{6.2 \nameref{subsec:data_collect}} \dotfill \pageref{subsec:data_collect}
        \item \textcolor{eccvblue}{6.3 \nameref{subsec:label_map}} \dotfill \pageref{subsec:label_map}
        \item \textcolor{eccvblue}{6.4 \nameref{subsec:adverse_condition}} \dotfill \pageref{subsec:adverse_condition}
         \item \textcolor{eccvblue}{6.5 \nameref{subsec:license}} \dotfill \pageref{subsec:license}
    \end{itemize}
    
    \item \textcolor{eccvblue}{\textbf{7. \nameref{sec:supp_implement}}} \dotfill \pageref{sec:supp_implement}
    \begin{itemize}
        \item \textcolor{eccvblue}{7.1 \nameref{subsec:lidar_config}} \dotfill \pageref{subsec:lidar_config}
        \item \textcolor{eccvblue}{7.2 \nameref{subsec:corruption_gen}} \dotfill \pageref{subsec:corruption_gen}
        \item \textcolor{eccvblue}{7.3 \nameref{subsec:hyperparam}} \dotfill \pageref{subsec:hyperparam}
    \end{itemize}
    
    \item \textcolor{eccvblue}{\textbf{8. \nameref{sec:supp_quantitative}}} \dotfill \pageref{sec:supp_quantitative}
    \begin{itemize}
        \item \textcolor{eccvblue}{8.1 \nameref{subsec:seg_quant}} \dotfill \pageref{subsec:seg_quant}
        \item \textcolor{eccvblue}{8.2 \nameref{subsec:det_quant}} \dotfill \pageref{subsec:det_quant} 
    \end{itemize}
    
    \item \textcolor{eccvblue}{\textbf{9. \nameref{sec:supp_qualitative}}} \dotfill \pageref{sec:supp_qualitative}
    \begin{itemize}
        \item \textcolor{eccvblue}{9.1 \nameref{subsec:seg_qual}} \dotfill \pageref{subsec:seg_qual}
        \item \textcolor{eccvblue}{9.2 \nameref{subsec:det_qual}} \dotfill \pageref{subsec:det_qual}
    \end{itemize}

\item \textcolor{eccvblue}{\textbf{10. \nameref{sec:proof}}} \dotfill \pageref{sec:proof}
    \begin{itemize}
        \item \textcolor{eccvblue}{10.1 \nameref{subsec:proof_thm}} \dotfill \pageref{subsec:proof_thm}
        \item \textcolor{eccvblue}{10.2 \nameref{subsec:proof_rmk}} \dotfill \pageref{subsec:proof_rmk}
    \end{itemize}

    \item \textcolor{eccvblue}{\textbf{11. \nameref{sec:discussion}}} \dotfill \pageref{sec:discussion}
    \begin{itemize}
        \item \textcolor{eccvblue}{11.1 \nameref{subsec:limitation}} \dotfill \pageref{subsec:limitation}
        \item \textcolor{eccvblue}{11.2 \nameref{subsec:potential_societal_impact}} \dotfill \pageref{subsec:potential_societal_impact}
    \end{itemize}
    
    \item \textcolor{eccvblue}{\textbf{12. \nameref{sec:supp_acknowledge}}} \dotfill \pageref{sec:supp_acknowledge}

\end{itemize}
