# Supplementary material for: Is Your LiDAR Placement Optimized for 3D Scene Understanding?
Source: arXiv:2403.17009 source file (2024-10-30)
Supplement: Supplementary file 2 [file dataset_det.tex]

\begin{table}[!t]
\caption{Comparisons between \textbf{Place3D} and popular driving perception datasets for the LiDAR semantic segmentation and 3D object detection tasks.}
\label{tab:lidar_datasets}
\vspace{-0.2cm}
\centering
\resizebox{\textwidth}{!}{
\begin{tabular}{r|p{1.765cm}<{\centering}p{1.765cm}<{\centering}p{1.765cm}<{\centering}p{1.765cm}<{\centering}p{1.765cm}<{\centering}}

\toprule
\textbf{}   & \textbf{nuScenes} & \textbf{Waymo} & \textbf{KITTI} & \textbf{Lyft} & \textbf{Place3D}
\\
\midrule\midrule
Detection Classes & 10 &  & 3 & 9 &  3
\\
Segmentation Classes & 16 &  & 19 & - &  21
\\
\# of Scenes      & 1000 &  & - & $162 \times 10^3$ &  340
\\
\# of Instances &  &  & 80,256 &  & $7.1 \times 10^4$
\\
Points Per Frame & $3.0 \times 10^4$ &  &  &  & $1.6 \times 10^4$
\\
\# of LiDAR Channels & 32 & 64 & 64 & 40 & 64
\\
Vertical FOV & [-30.0, 10.0] & [-17.6, 2.4] & [-24.8, 2.0] &  & [-24.8, 2.0]
\\
% Horizontal FOV & 360 &  & 120 &  & 360
% \\
Placement Strategy & \textcolor{place3d_red}{Single} & \textcolor{place3d_red}{Single} & \textcolor{place3d_red}{Single} & \textcolor{place3d_red}{Single} & \textcolor{place3d_blue}{Multiple}
\\
Adverse Conditions & \textcolor{place3d_red}{No} & \textcolor{place3d_red}{No} & \textcolor{place3d_red}{No} & \textcolor{place3d_red}{No} & \textcolor{place3d_blue}{Yes}
\\
\bottomrule
\end{tabular}
}
\end{table}
